# Supplementary material for: Representing Long Volumetric Video with Temporal Gaussian Hierarchy
Source: arXiv:2412.09608 source file (2024-12-12)
Supplement: Supplementary file 1 [file supp.tex]

\documentclass[acmtog,anonymous,review]{acmart}

\input{macros}

\begin{document}

\title{Supplementary Material for Long Volumetric Video}

\input{content/00_abstract}

\maketitle

\bibliographystyle{ACM-Reference-Format}
\bibliography{reference}
\appendix
\input{content/09_supplementary}

\end{document}
